# Supplementary material for: Liquid phase stabilization versus bubble formation at a nanoscale-curved interface
Source: arXiv:1610.09325 source file (2017-06-21)
Supplement: Supplementary file 1 [file Supplemental_Materials.pdf]

# Supplemental materials for: Liquid phase stabilization versus bubble nucleation at a nanoscale-curved interface

Jarrod Schiffbauer[1,*] and Tengfei Luo[1,2,†]

[1] *University of Notre Dame, Department of Aerospace and Mechanical Engineering, Notre Dame, IN, 46556*

[2] *Center for Sustainable Energy at Notre Dame, Notre Dame, IN, 46556*

(Dated: June 21, 2017)

## Abstract

Additional notes on the models in main text.

PACS numbers: 05.70.Np, 05.70.Ln, 47.55.db, 65.20.-w, 68.03.Fg, 68.03.Cd

*Electronic address: jschiffb@nd.edu

†Electronic address: tluo@nd.edu

## I. GIBBS MODEL

Eqn. 1 of the main text was obtained by considering the difference in Gibbs energy per mole between the final state of thin vapor layer + bulk liquid + solid-vapor + liquid-vapor interfaces and the initial state of bulk liquid + solid-liquid interface, then multiplying by the number of moles of vapor contained in a thin spherical shell of thickness $\tilde{\delta r}$. Where possible, values were used for Argon, obtained from [1] for the fluid. The fluid-solid interface parameter ranges were inferred from a combination of experimental and theoretical data in the literature, principally [2].

## II. NON-EQUILIBRIUM MODEL

The (dimensional) governing equations are as follows, with the ‘ ˜ ’ denoting dimensional variables: Mass transport is given by $\partial_t \tilde{n} + \nabla \cdot (\tilde{n}\tilde{\mathbf{v}}) = 0$ where $\tilde{n}$ is the number density. The fluid velocity, $\tilde{\mathbf{v}}$ is obtained from, $M\tilde{n}\left(\partial_t \tilde{\mathbf{v}} + \tilde{\mathbf{v}} \cdot \nabla \tilde{\mathbf{v}}\right) = -\nabla \cdot \left(\tilde{\mathbb{P}} - \tilde{\mathbb{D}}\right)$ with molecular mass, $M$, pressure, and viscous dissipation tensors, $\tilde{\mathbb{P}}$ and $\tilde{\mathbb{D}}$ respectively. The temperature is governed by, $\tilde{c}_v \left(\partial_t \tilde{T} + \tilde{\mathbf{v}} \cdot \nabla \tilde{T}\right) = -\tilde{\ell} \nabla \cdot \tilde{\mathbf{v}} + \nabla \left(\lambda \nabla \tilde{T}\right) + \tilde{\mathbb{D}} : \nabla \tilde{\mathbf{v}}$ with thermal conductivity, $\lambda$, and the Clayperon coefficient defined $\tilde{\ell} = \tilde{T}\left(\partial \tilde{P}_{bulk}/\partial \tilde{T}\right)_n$. Element-wise, the dissipation tensor is $\tilde{D}_{i,j} = \eta\left(\partial_i \tilde{v}_j + \partial_j \tilde{v}_i - \frac{2}{3}\nabla \cdot \tilde{\mathbf{v}}\hat{\delta_{i,j}}\right) + \mu \nabla \cdot \tilde{\mathbf{v}}\hat{\delta_{i,j}}$, where $\eta$ and $\mu$ are the shear and bulk viscosities, and $\hat{\delta_{i,j}}$ is the Kronnecker delta.

The pressure tensor is defined with a gradient contribution to the free energy density [3, 4], with elements $\tilde{P}_{i,j} = \left[\tilde{n}k_B\tilde{T}/(1-\Omega_o\tilde{n}) - \varepsilon\Omega_o\tilde{n}^2 - C\tilde{T}\tilde{n}\nabla^2\tilde{n} + C\tilde{T}\left(\nabla\tilde{n}\right)^2\right]\hat{\delta}_{i,j} + C\tilde{T}\partial_i\tilde{n}\partial_j\tilde{n}$ where $\Omega_o$ and $\varepsilon$ are respectively the Lennard-Jones volume and well-depth, and $k_B$ is the Boltzmann constant.

The specific heat is $\tilde{c}_V = 3k_B\tilde{n}/2$, and the Clayperon coefficient is obtained from the bulk (dimensionless) pressure $P = nT/(1-\alpha n) - \frac{27}{8}\alpha n^2$. We assume $\eta \approx \mu = \nu M\tilde{n}$ with a constant kinematic viscosity, $\nu$, for simplicity. This also permits control of viscous dissipation in a convenient way. The thermal conductivity is taken to be $\lambda = k_B\nu\tilde{n}$, following [4].

To simulate evolution of an initially uniform fluid of temperature $T = 0.56$ and density $n = 1.005$ in contact with a nanocurved surface of infinite heat capacity and infinite interfa-

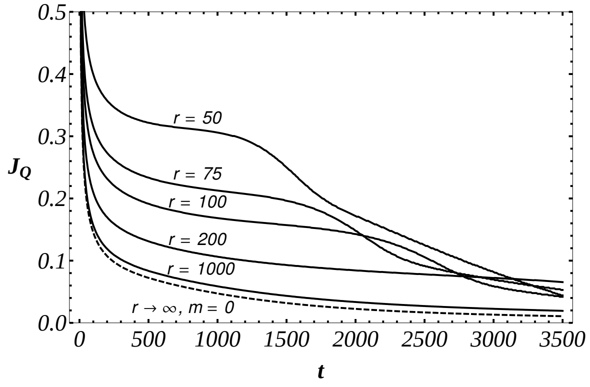


FIG. 1: Heat flux into hot boundary for varying inner radius $r_{np}$. The calculation uses a fixed kinematic viscosity $1.67 \times 10^{-6}$ m$^2$/s, with $\alpha = 0.208$, $\beta = 47.192$, $\delta = 10^{-3}$, and $\chi = -10^{-3}$.

cial conductance (see Fig. 1 main text), the governing equations are solved numerically on a 1D grid for several values of boundary radius $r$ with $m = 0, 2$. The boundary conditions are $T(r, t) = 0.85$ and $T(d + r, t) = 0.56$, $P(x, 0) = P(d + r, t) = 0.0059$ (about 0.7 MPa), $n(d + r, t) = 1.005$, $v = 0$ at both interfaces.

For preliminary runs, we choose parameters from the lower end of the range, $\delta = 10^{-9}$ and $\delta = 10^{-3}$, and $\chi = -10^{-3}$ (weakly hydrophilic surface with low capillary contribution). The input heat flux, $-\beta n \partial_x T(x = r)$ is evaluated as an average over the first few grid points, and plotted in Fig. 1. Overall, the heat flux into interfaces with smaller radii is higher, as might be expected from purely geometric effects, and the heat flux response with increasing radius is seen to approach the planar $m = 0$ case in the limit $r \to \infty$.

---

[1] *Thermophysical properties of fluid systems*, accessed: 2016-09-30, URL `http://http://webbook.nist.gov/chemistry/fluid/`.

[2] A. Adamson and A. Gast, *Physical Chemistry of Surfaces* (Wiley-Interscience, 1997).

[3] A. Onuki, Phys. Rev. E **75**, 036304 (2007).

[4] R. Teshigawara and A. Onuki, Phys. Rev. E **82**, 021603 (2010).
